# Supplementary material for: Pythia: Grammar-Based Fuzzing of REST APIs with Coverage-guided Feedback and Learning-based Mutations
Source: arXiv:2005.11498 source file (2020-05-23)
Supplement: Supplementary file 1 [file appendix.tex]

\section*{Appendix}
\F\ref{fig:restler} shows the complete \restler coverage over the complete
$48$h of fuzzing ($56$for ``Issues \& Notes) for each experiment.

\begin{figure*}[h]
    \begin{minipage}{\textwidth}
    \centering
    \subfigure{
        \includegraphics[width=0.31\textwidth]{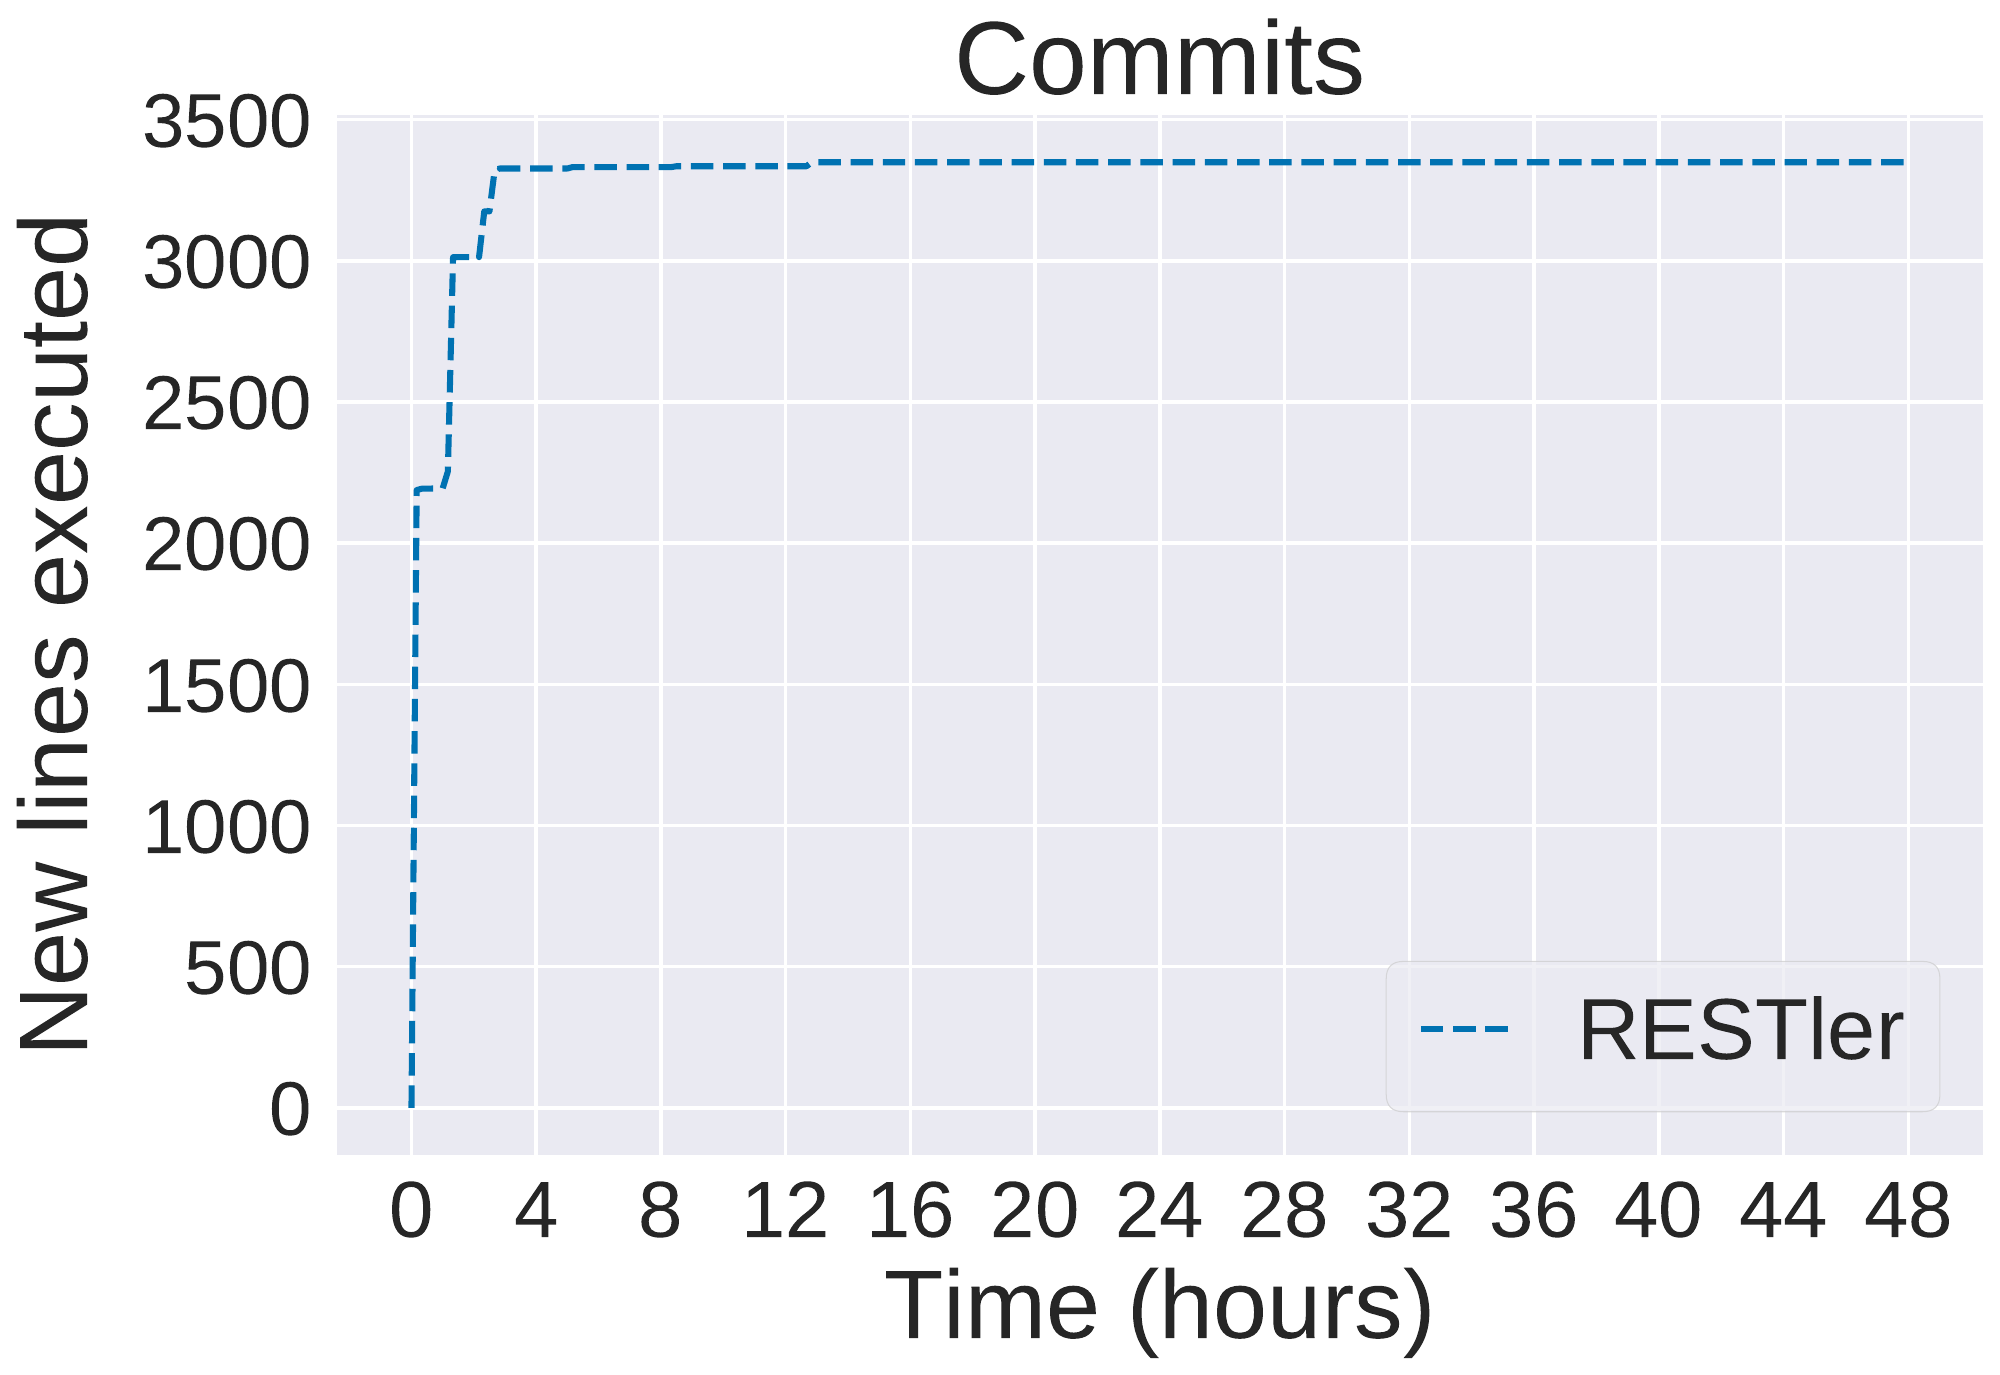}
    }
    \subfigure{
        \includegraphics[width=0.31\textwidth]{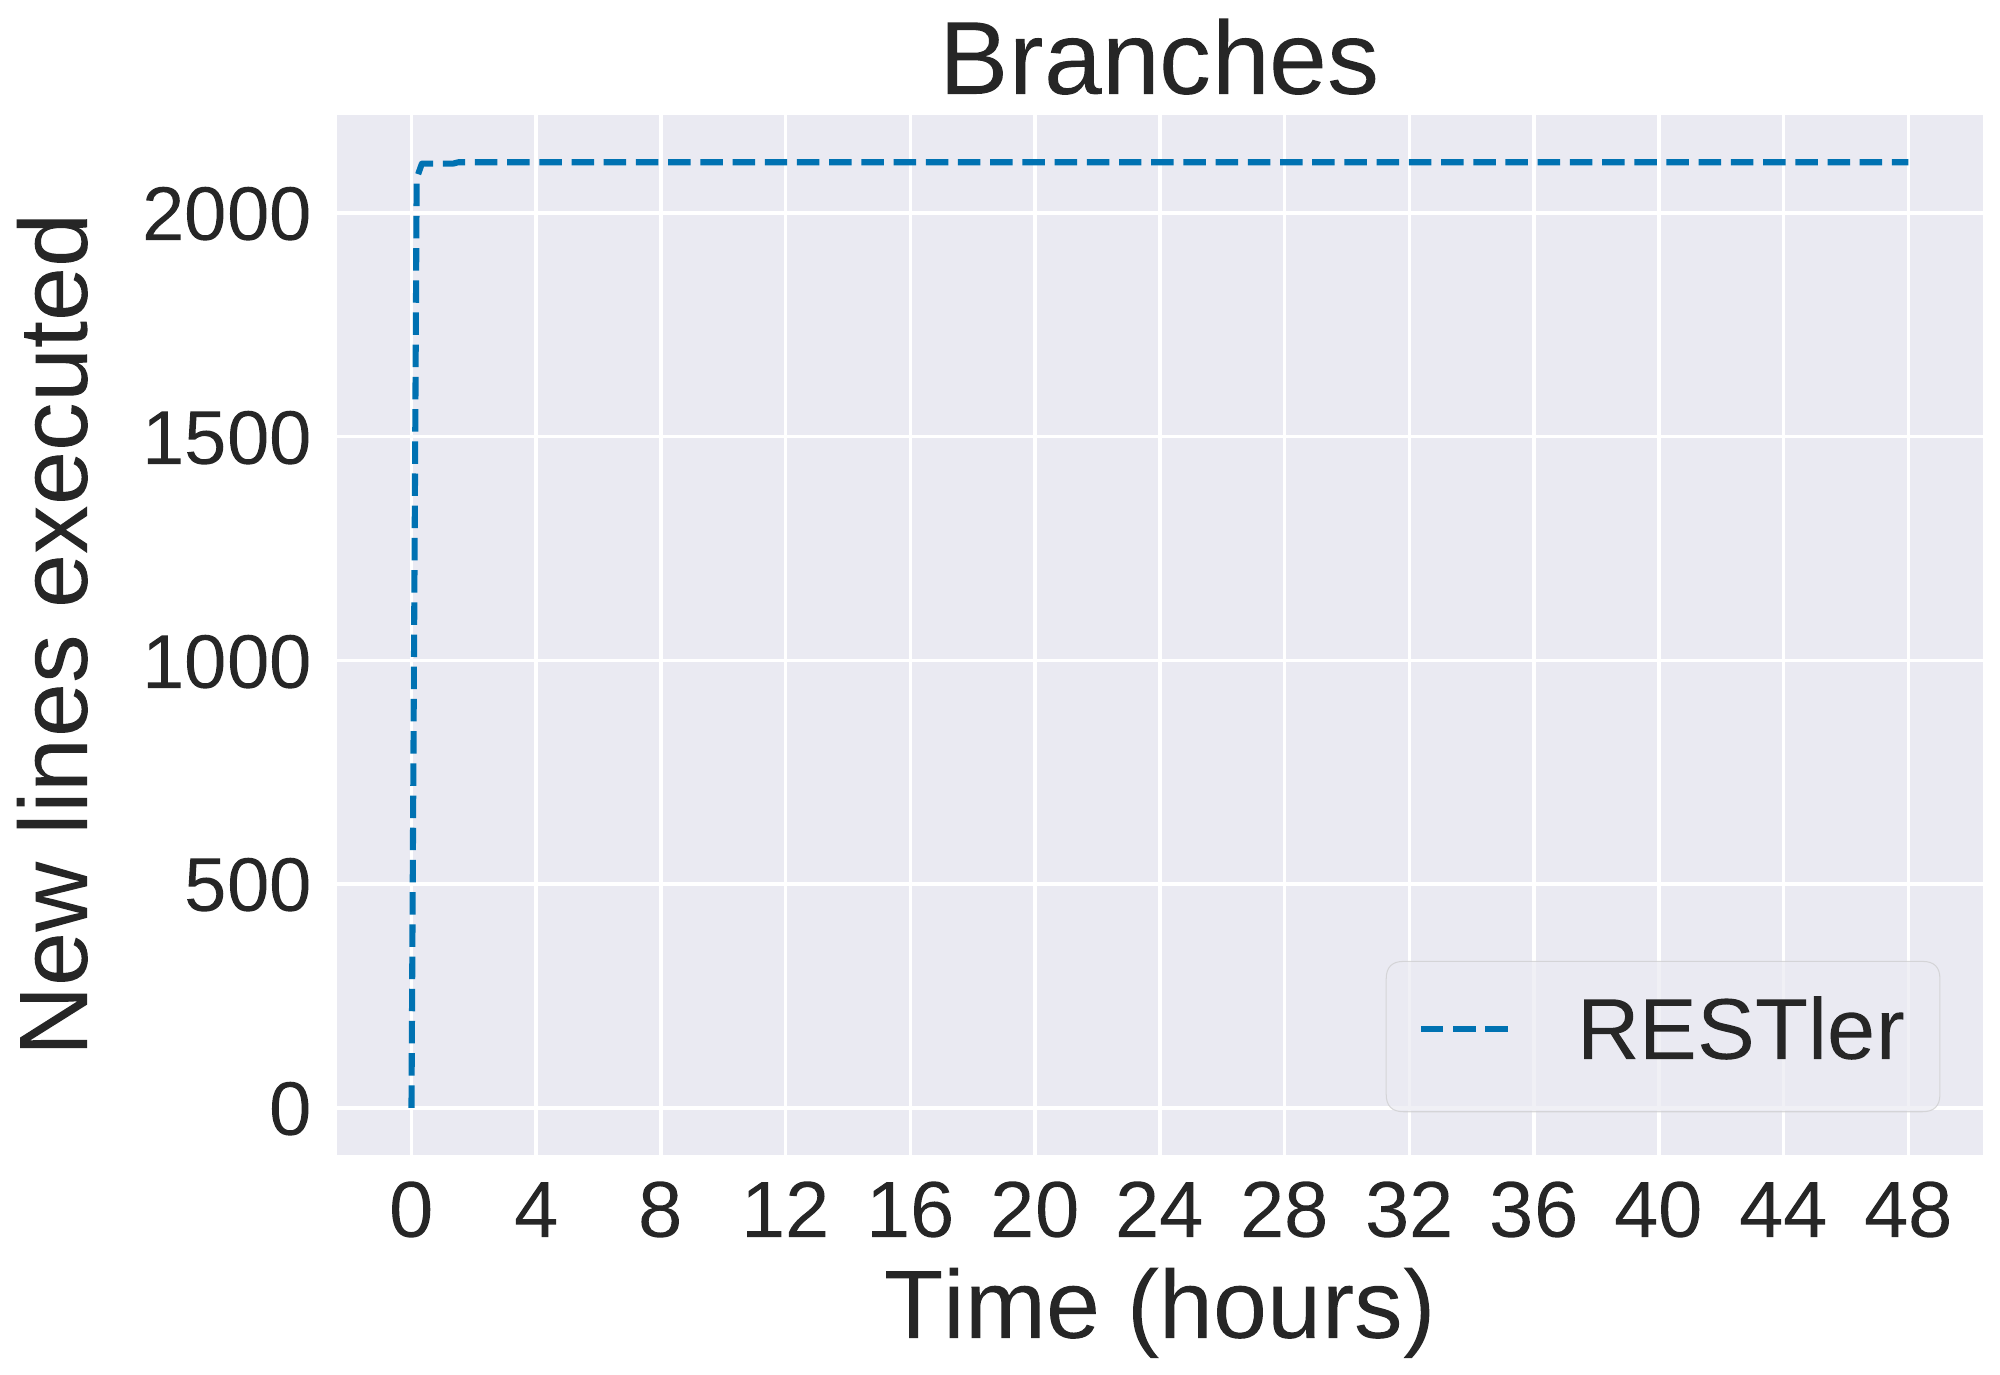}
    }
    \subfigure{
        \includegraphics[width=0.31\textwidth]{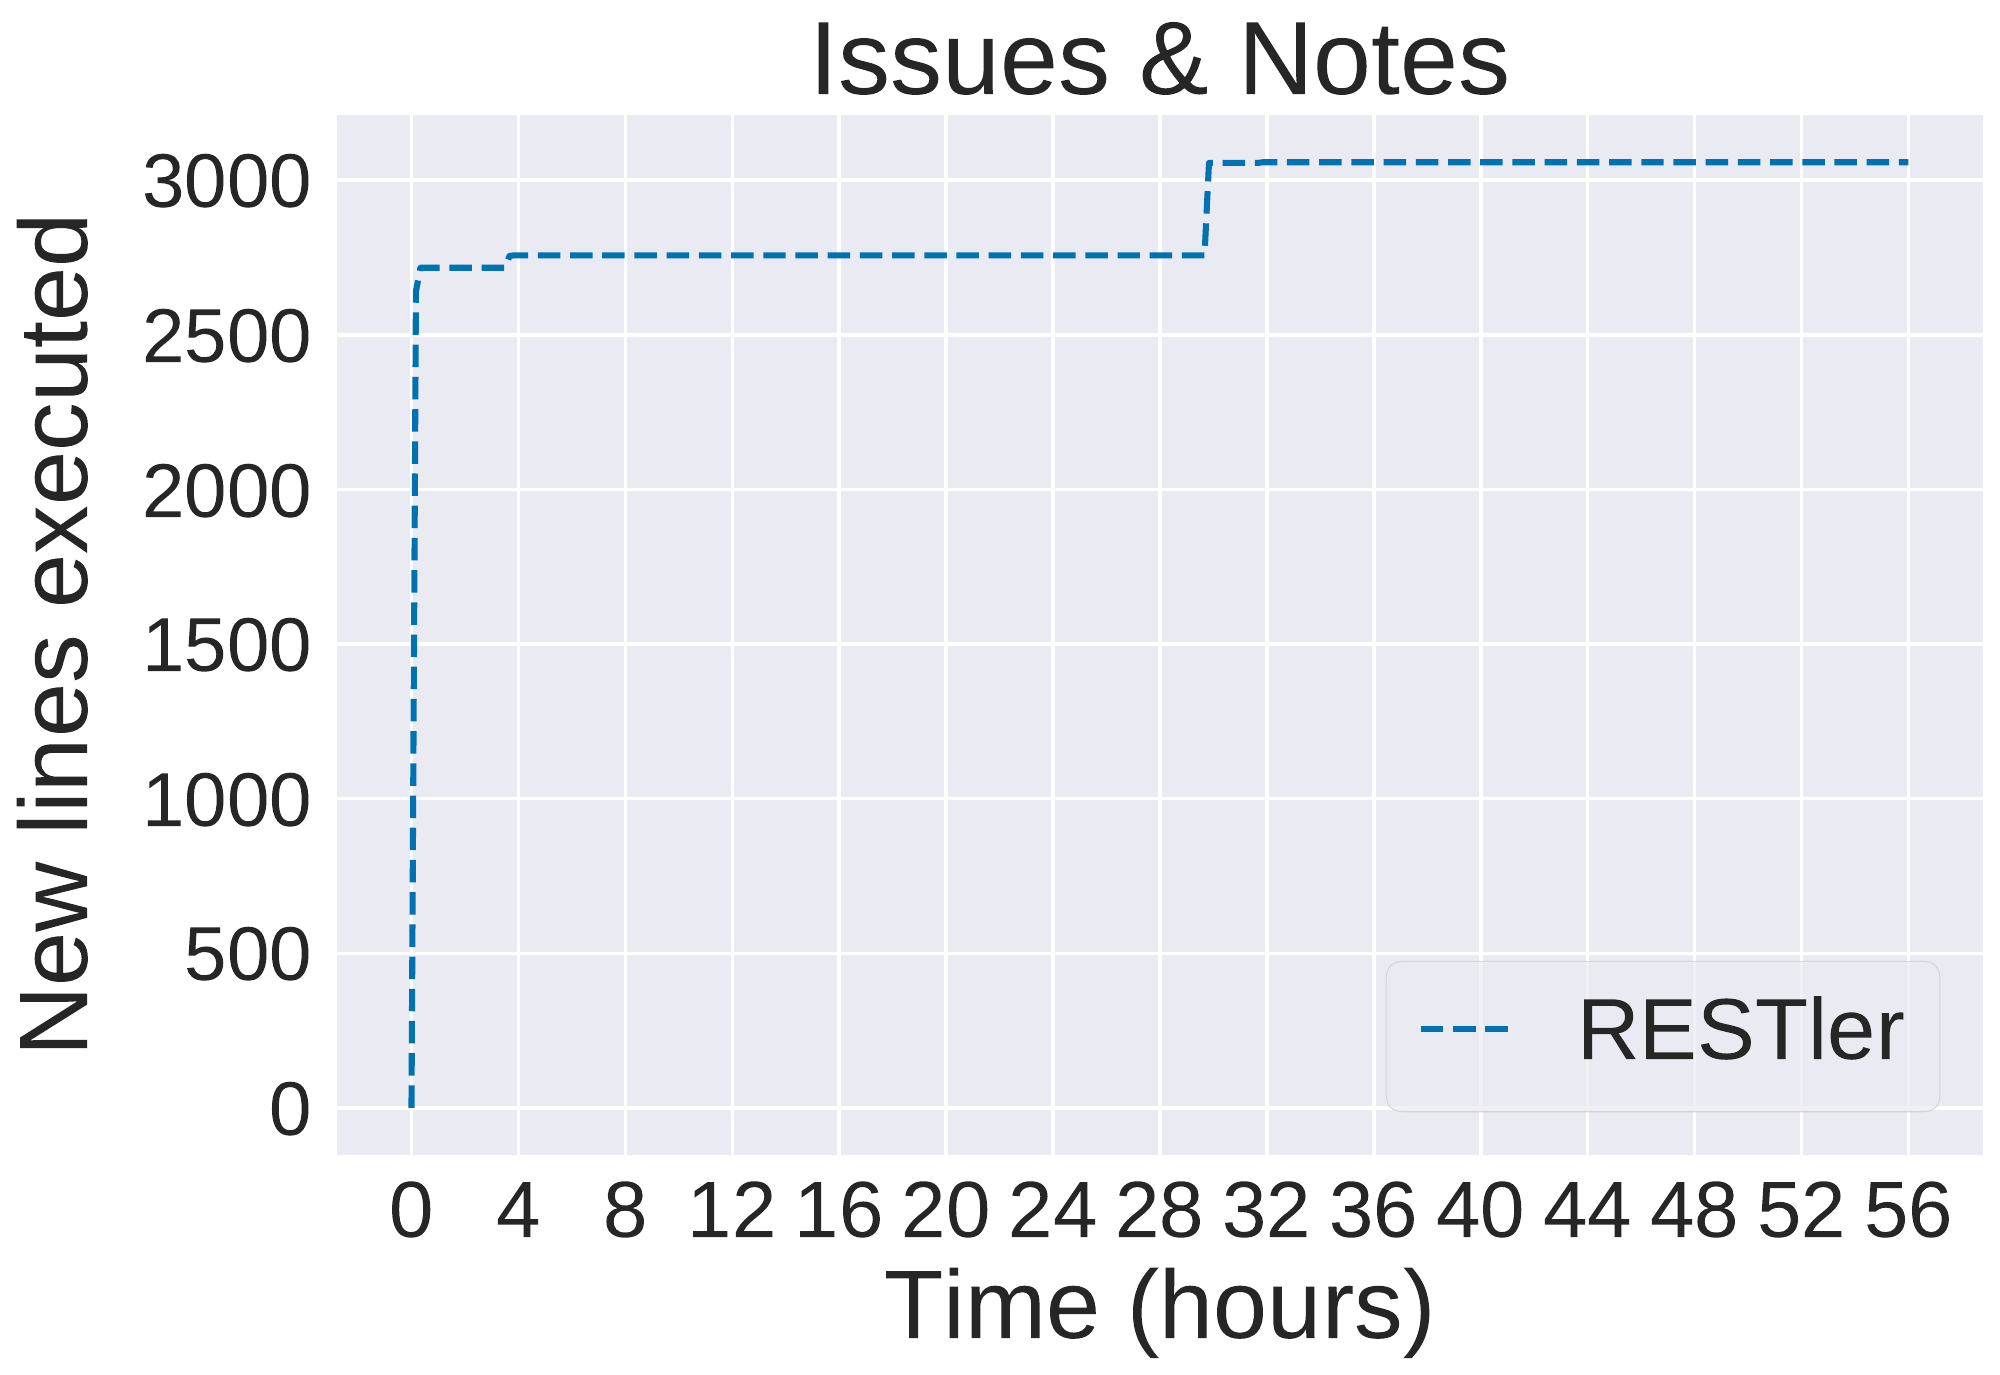}
    }
    \medskip
    \subfigure{
        \includegraphics[width=0.31\textwidth]{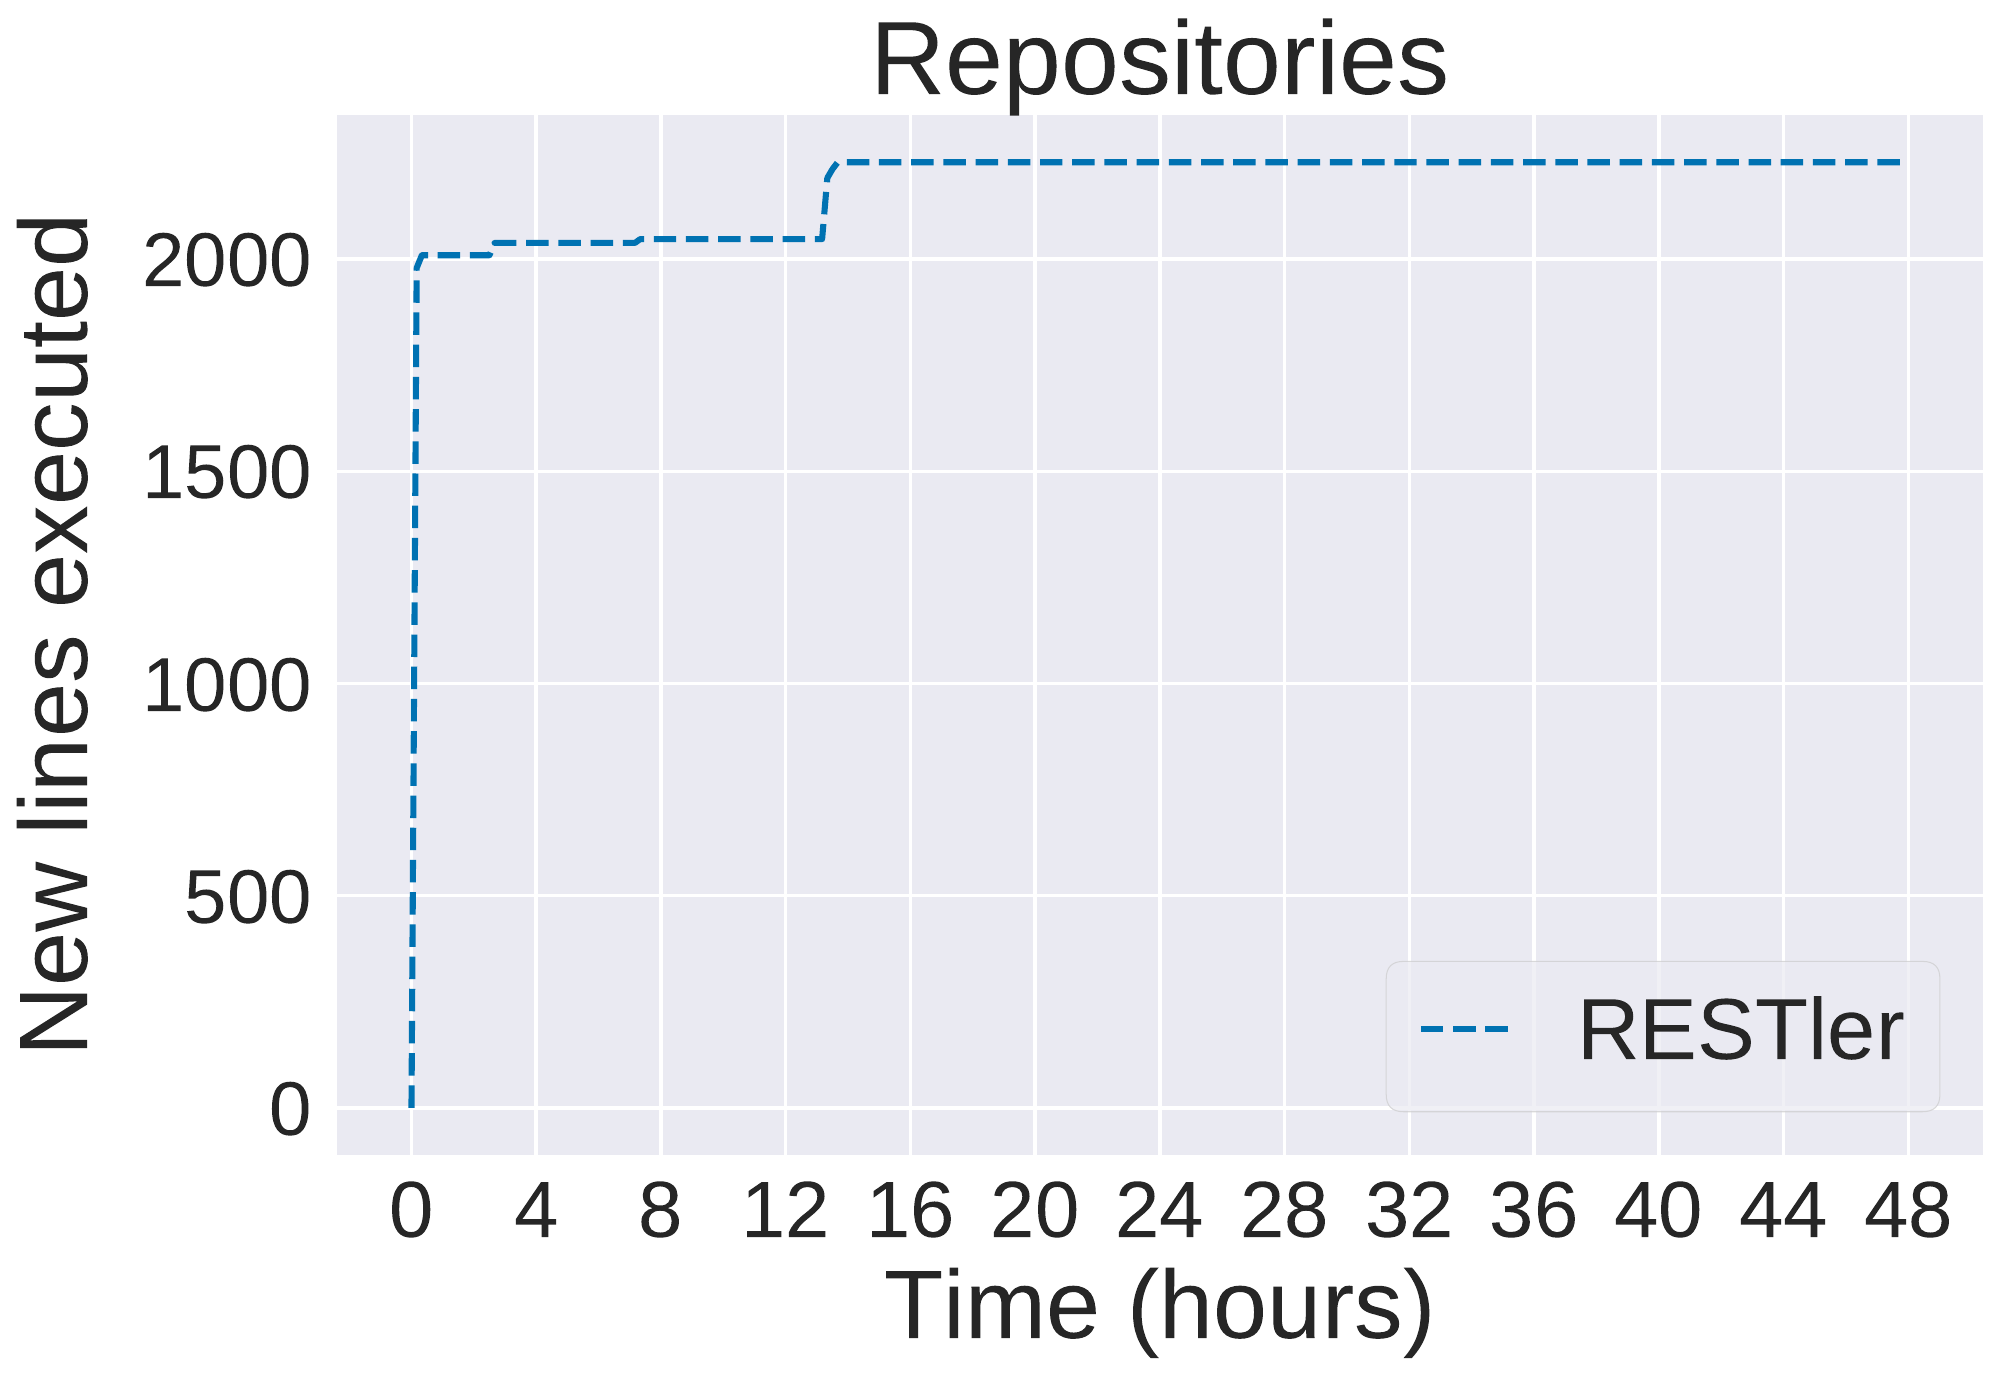}
    }
    \subfigure{
        \includegraphics[width=0.31\textwidth]{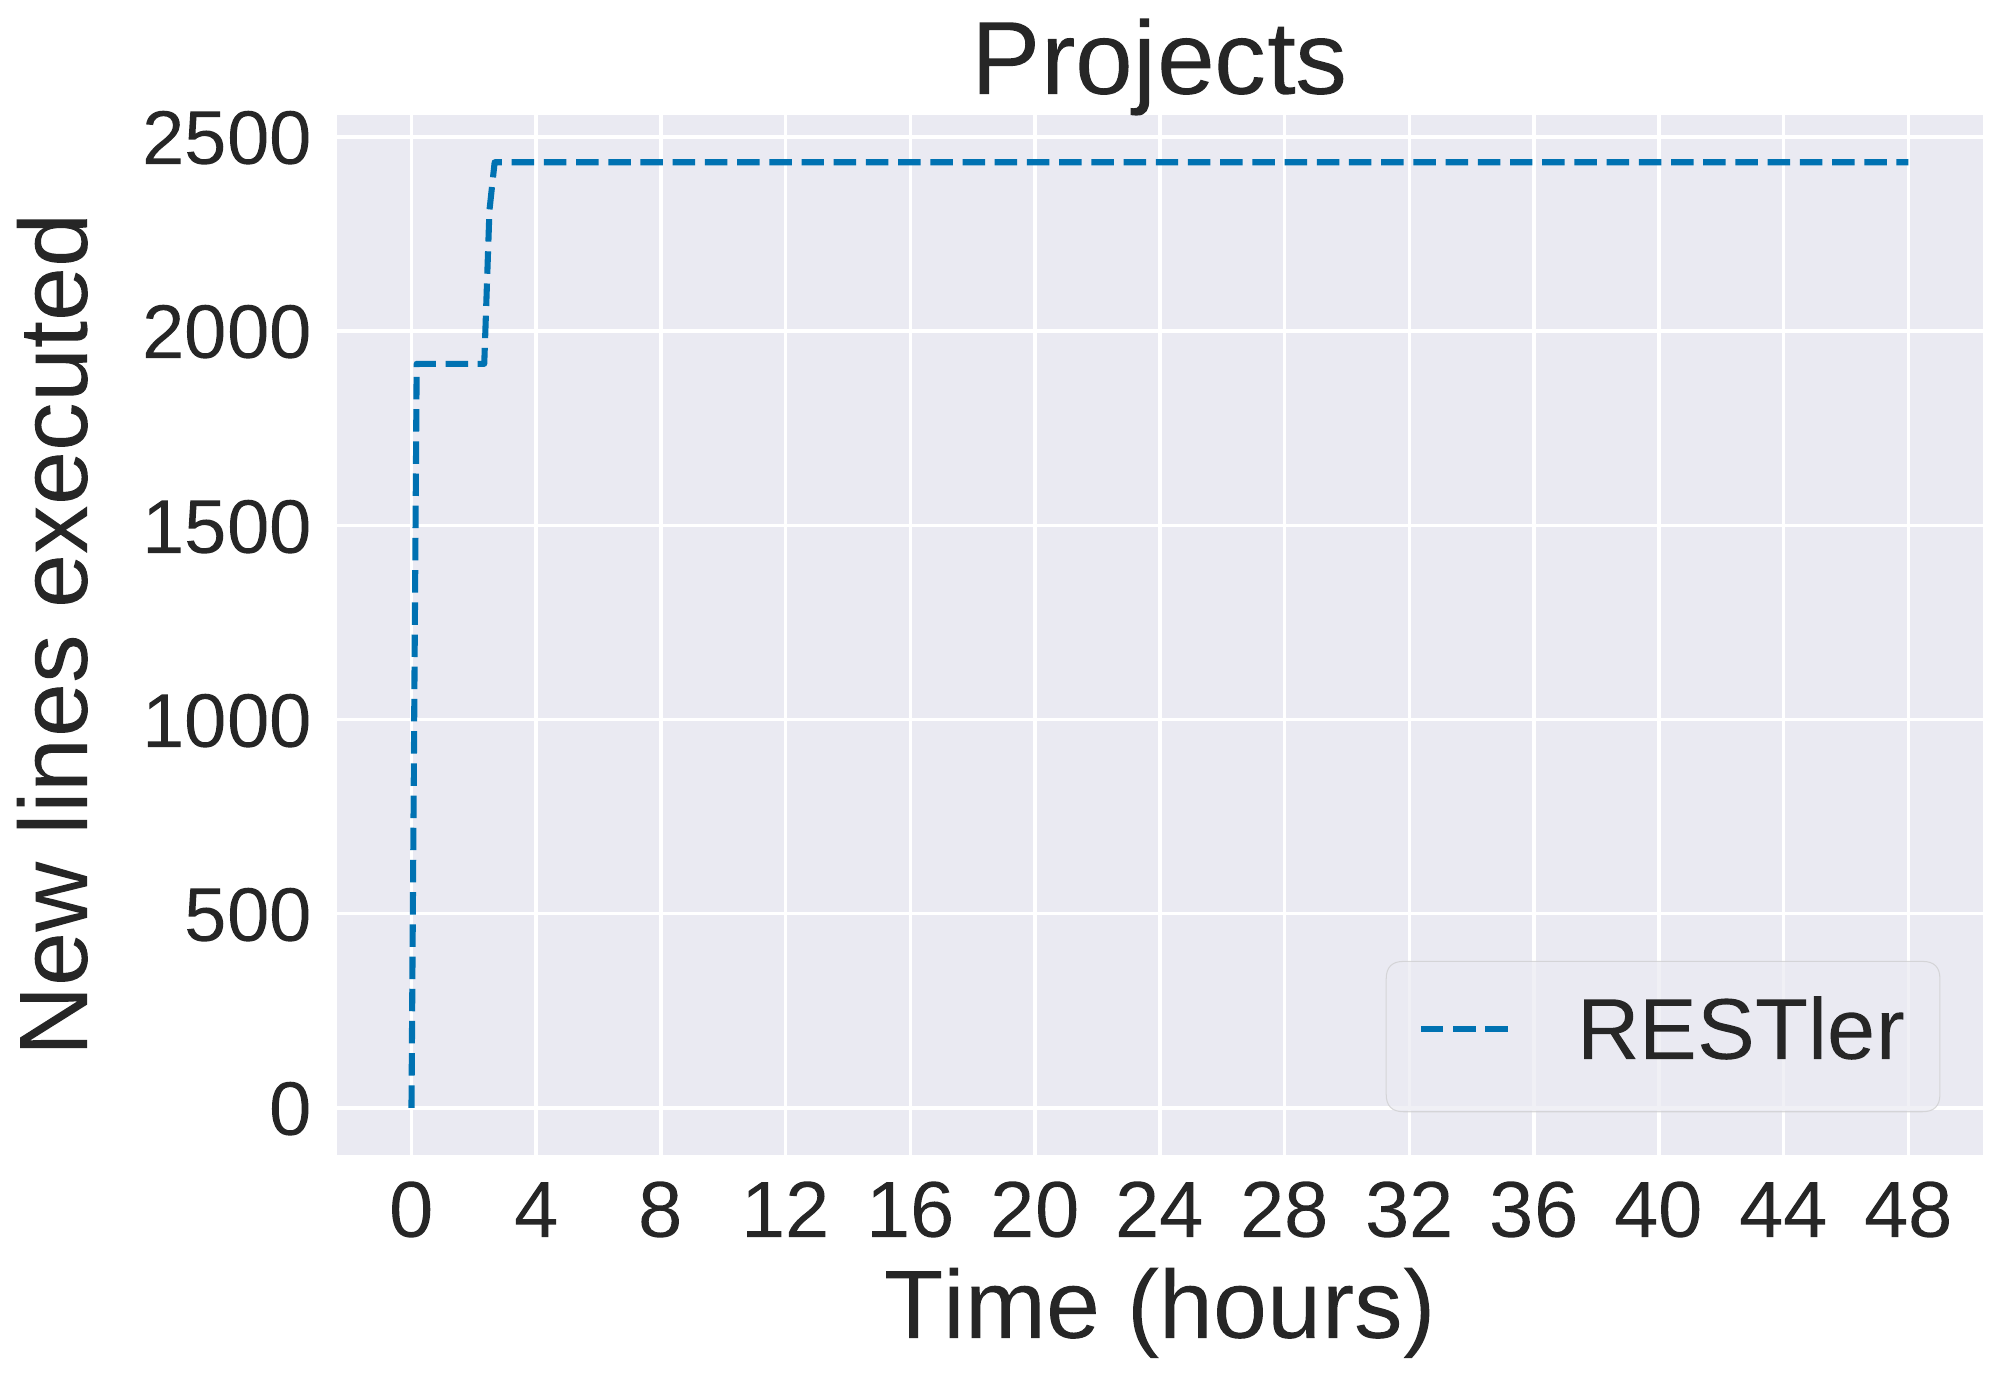}
    }
    \subfigure{
        \includegraphics[width=0.31\textwidth]{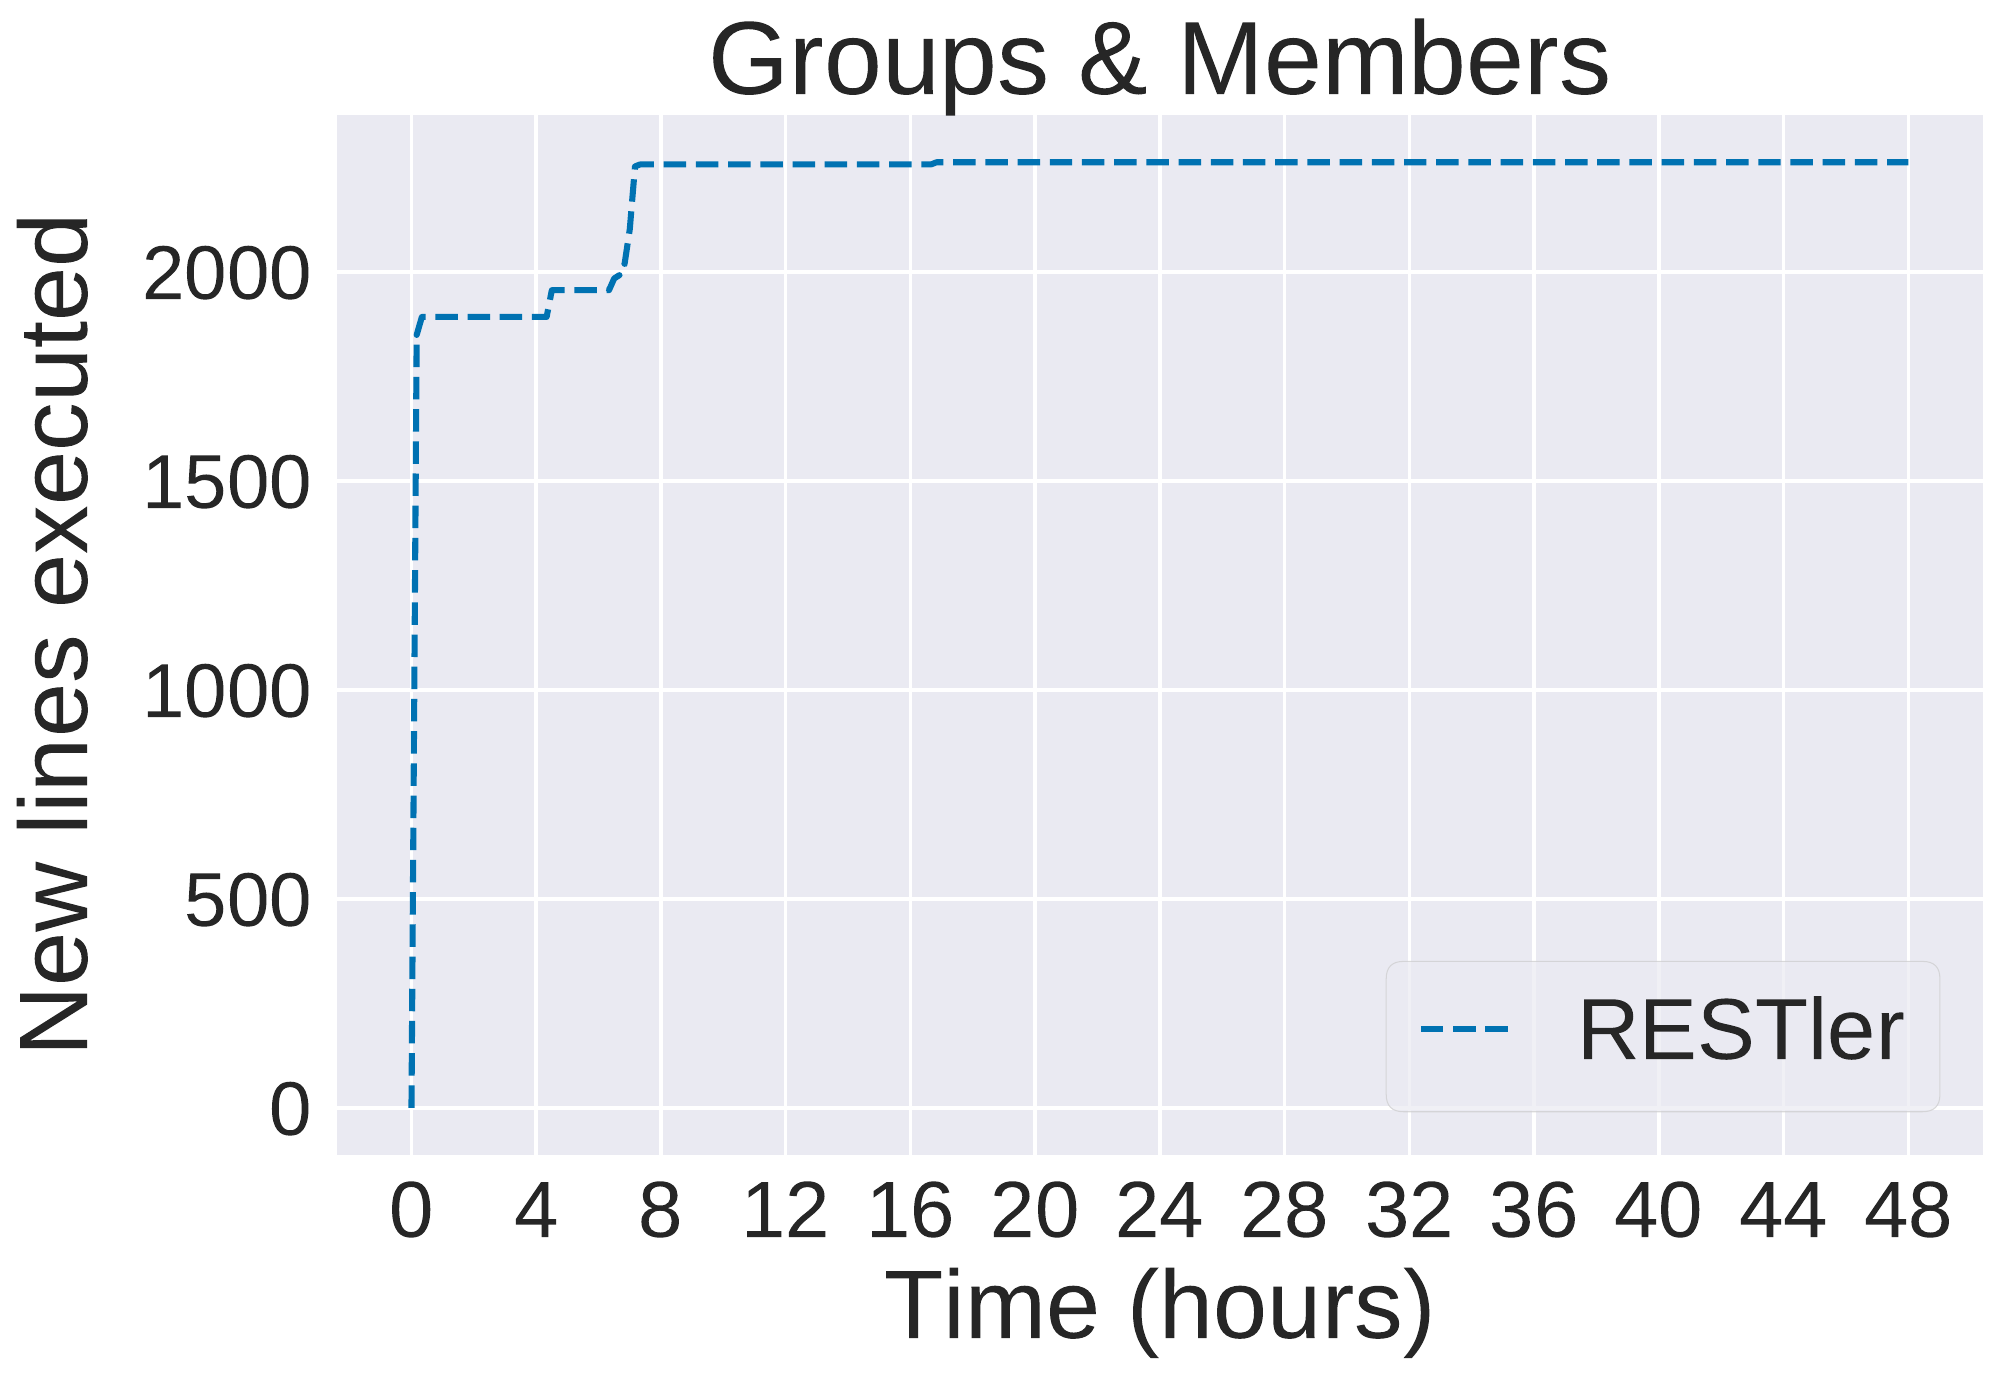}
    }
    \caption{
        {\bf \restler coverage.} Shows the complete \restler coverage over the
        total $48$h of fuzzing.}
    \label{fig:restler}
    \end{minipage}\\[1em]
\end{figure*}
